# Supplementary material for: Quantifying Hidden Symmetry in the Tetragonal CH$_3$NH$_3$PbI$_3$ Perovskite
Source: arXiv:2301.11281 ancillary file (2023-01-26)
Supplement: Supplementary file 1 [file Hidden_symmetry_Supplementary.pdf]

# Supporting Information: Quantifying Hidden Symmetry in the Tetragonal $CH_3NH_3PbI_3$ Perovskite

Kuntal Talit and David A. Strubbe*

*Department of Physics, University of California, Merced, 5200 N. Lake Rd., Merced, CA 95343*

E-mail: dstrubbe@ucmerced.edu

## Calculated symmetry of the structure using FINDSYM

Table S1: Tetragonal (I4cm) MAPI symmetry of the entire structure and only the Pb-I cage, calculated using FINDSYM.[S1,S2]

| Tetragonal MAPI | Tolerance in lattice (Å) | Tolerance in atomic positions (Å) | Calculated symmetry |
|---|---|---|---|
| Complete Structure | 0.001 | 0.001 | no symm. |
| | 0.2 | 0.2 | $C_s$ |
| | 0.5 | 0.5 | $C_s$ |
| Pb-I cage only | 0.01 | 0.01 | $C_s$ |
| | 0.01 | 0.1 | $C_s$ |
| | 0.1 | 0.1 | $C_s$ |
| | 0.1 | 0.2 | $C_{2h}$ |
| | 0.1 | 0.3 | $C_{2v}$ |
| | 0.1 | 0.4 | $D_{4h}$ |

## Computational method

We have studied two different tetragonal structures, one is quasi-I4cm[S3] and the other is quasi-I4/mcm.[S4] We did a full variable-cell structural relaxation of both the initial structures

using local density approximation[S5] (LDA) with the Perdew-Wang (PW) parametrization[S6] for the exchange correlation potential. We have used scalar relativistic optimized norm-conserving Vanderbilt (ONCV) pseudopotentials[S7] from Pseudō Dōjō[S8]) (NC SR ONCVPSP v0.4) with standard accuracy. A half-shifted 5× 5× 4 Monkhorst-Pack grid is used for Brillouin zone sampling along $x$, $y$, and $z$ directions of the crystallographic axes with energy cutoff of 80 Ry for the wave functions. Variable-cell relaxation is done using a 0.5 kbar stress convergence threshold keeping total force per atom less than 1 meV/Å. Before deep diving into the symmetry of the tetragonal structure we have compared different functionals and compared the structural parameters. PBE with Grimme-D2 van der Waals corrections gives best results for structural parameters compared to the experimental results but we have chosen LDA because the Raman intensity can only be computed using it in Quantum ESPRESSO. An earlier report suggests that LDA without van der Waals correction can still be good to calculate Raman and IR frequency and intensity for orthorhombic MAPI.[S9] We have calculated the stiffness matrix by applying uniaxial strain to these two structures and calculating the stress tensor using Quantum ESPRESSO. The dielectric and the electro-optic tensor is calculated using Quantum ESPRESSO `ph.x` code which uses density functional perturbation theory to calculate these tensors.

It is important to note that the phonon mode vectors that directly come out of the Quantum ESPRESSO dynmat.x code output are normalized to 0.1 and not normalized with the corresponding atomic masses and hence are not orthogonal to each other; they are just mode displacement vectors. To make these modes orthogonal mode eigenvectors we need to normalize them with corresponding atomic masses. This means we need to multiply each mode eigenvector with the corresponding mass of the atom and then normalize them to 1. Our method should work fine even if we do not normalize these modes with respect to mass but we normalized them properly before doing further calculations because this will help later to find the degeneracy in the modes.

# Calculated stiffness and dielectric tensors

Stiffness tensor (calculated values are in GPa)

$$\begin{pmatrix} C_{11} & C_{12} & C_{13} & & & \\ . & C_{11} & C_{13} & & & \\ . & . & C_{33} & & & \\ & & & C_{44} & & \\ & & & & C_{44} & \\ & & & & & C_{66} \end{pmatrix} \quad \begin{pmatrix} 28.95 & 19.98 & 10.27 & -0.71 & 0.00 & 0.34 \\ 19.92 & 28.94 & 10.27 & 0.01 & -0.71 & 0.34 \\ 10.27 & 10.27 & 44.15 & 0.44 & 0.49 & 0.75 \\ -0.71 & -0.01 & 0.46 & 3.84 & 0.40 & 0.40 \\ -0.03 & -0.72 & 0.49 & 0.40 & 3.84 & 0.40 \\ 0.34 & 0.32 & 0.76 & 0.40 & 0.41 & 12.34 \end{pmatrix}$$

tetragonal-(I) I4cm

$$\begin{pmatrix} C_{11} & C_{12} & C_{13} & & & \\ & C_{22} & C_{23} & & & \\ & & C_{33} & & & \\ & & & C_{44} & & \\ & & & & C_{55} & \\ & & & & & C_{66} \end{pmatrix} \quad \begin{pmatrix} 29.24 & 20.24 & 10.73 & 0.00 & 0.00 & -0.02 \\ 20.20 & 27.90 & 10.14 & 0.01 & 0.00 & -0.02 \\ 10.68 & 10.18 & 43.32 & -0.01 & 0.00 & 0.01 \\ 0.00 & 0.00 & 0.00 & 4.10 & 0.00 & 0.00 \\ 0.00 & 0.00 & 0.00 & 0.00 & 2.88 & 0.00 \\ 0.00 & 0.00 & 0.00 & 0.00 & 0.00 & 12.26 \end{pmatrix}$$

orthorhombic I4/mcm

Figure S1: Stiffness matrix calculated for quasi-I4cm and quasi-I4/mcm structures and compared with the tetragonal-(I)[S10] and orthorhombic symmetry.

$$\text{I4cm} \quad \epsilon_\infty = \begin{pmatrix} 5.941 & 0.037 & -0.013 \\ 0.037 & 5.941 & -0.013 \\ -0.013 & -0.013 & 5.978 \end{pmatrix} \quad \epsilon_0 = \begin{pmatrix} 18.065 & 0.173 & -0.146 \\ 0.173 & 18.066 & -0.146 \\ -0.146 & -0.146 & 16.513 \end{pmatrix}$$

$$\text{I4/mcm} \quad \epsilon_\infty = \begin{pmatrix} 5.962 & 0.000 & 0.000 \\ 0.000 & 5.932 & 0.000 \\ 0.000 & 0.000 & 6.071 \end{pmatrix} \quad \epsilon_0 = \begin{pmatrix} 18.257 & 0.000 & 0.000 \\ 0.000 & 18.152 & 0.001 \\ 0.000 & 0.001 & 16.613 \end{pmatrix}$$

Figure S2: Static dielectric tensors for quasi-I4cm and quasi-I4/mcm structures: $\epsilon_\infty$ includes only the electronic contribution and $\epsilon_0$ includes the electronic and ionic contributions.

# Norm of mode eigenvectors without H

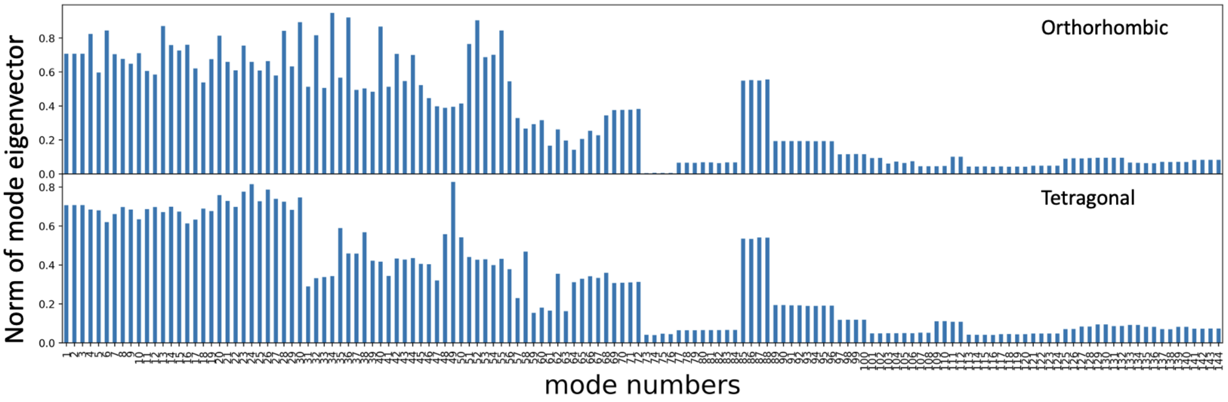


Figure S3: Norm of the vibrational mode eigenvectors for orthorhombic and tetragonal MAPI structures, excluding contributions from hydrogen atoms.

## Values of $\sum_{i=1}^{144} \chi_i^2$ for I4cm and I4/mcm structures.

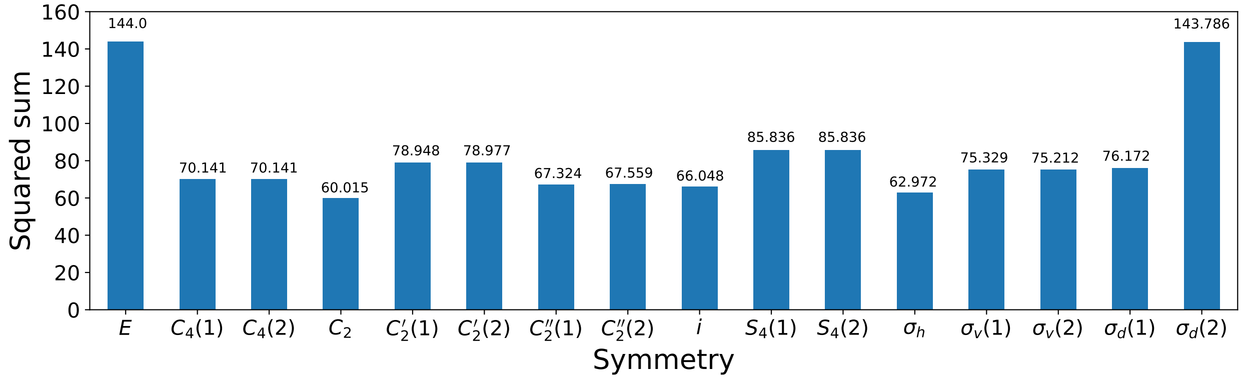


(a) I4cm

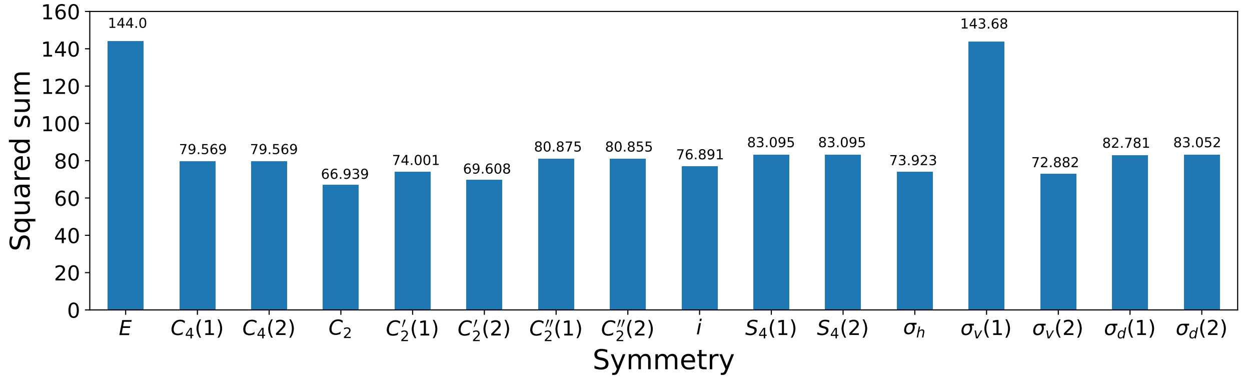


(b) I4/mcm

Figure S4: The sum of the mode characters squared ($\chi^2$ for non-degenerate modes and $2(|\chi_1 + \chi_2| - 1)^2$ for doubly degenerate modes) for each symmetry class over all the phonon modes of tetragonal MAPI.

# Test results for for $TiO_2$ and Orthorhombic MAPI

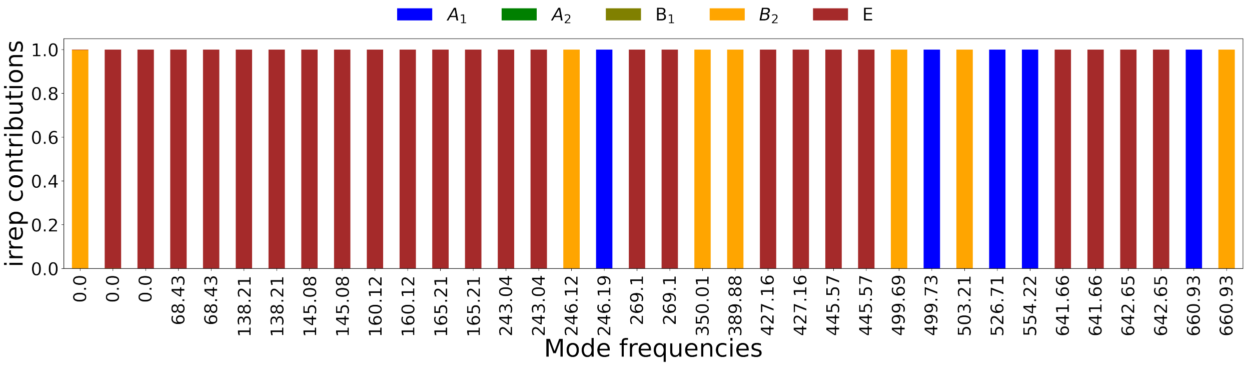


(a) $TiO_2$

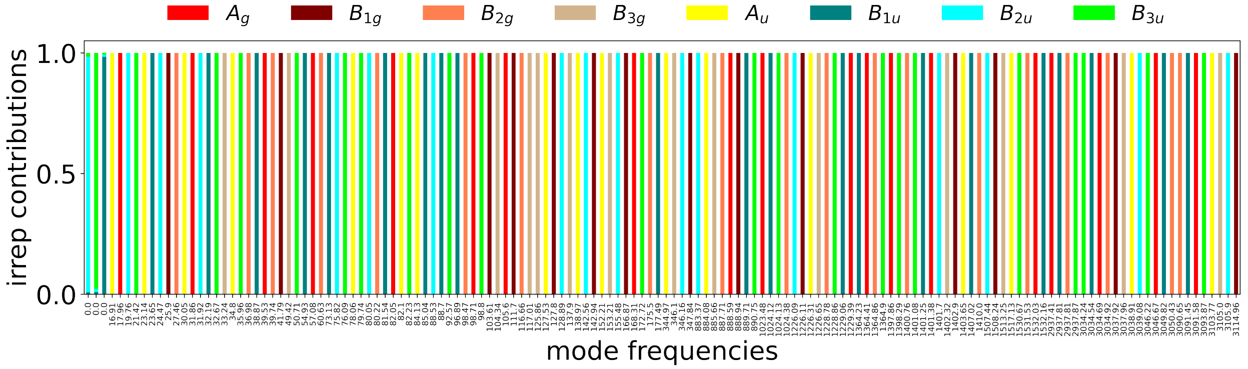


(b) Orthorhombic MAPI

Figure S5: Contribution of irreducible representations for (a) $TiO_2$ and (b) orthorhombic MAPI without considering the H atoms in the structure, calculated using our analytical method. Mode frequencies are in $cm^{-1}$.

# Optimized tetragonal I4cm and I4/mcm structures

Table S2: `alat` is in Bohr units.

**I4cm**

| | | | |
|---|---|---|---|
| **CELL_PARAMETERS (alat=16.43165998)** | | | |
| | 0.979807479 | 0.000365594 | -0.002594346 |
| | 0.001128900 | 0.979811798 | -0.001516903 |
| | 0.008879481 | 0.007174722 | 1.451802233 |
| **ATOMIC_POSITIONS (crystal)** | | | |
| C | 0.028975534 | 0.500796712 | 0.249292862 |
| C | 0.536063304 | 0.043885171 | 0.247443711 |
| C | 0.043862358 | 0.536134568 | 0.747400854 |
| C | 0.500795660 | 0.028933460 | 0.749328121 |
| N | 0.922539300 | 0.611362428 | 0.196294988 |
| N | 0.426905680 | 0.931390920 | 0.199888773 |
| N | 0.931401426 | 0.426918517 | 0.699871295 |
| N | 0.611387713 | 0.922528506 | 0.696316058 |
| H | 0.656320145 | 0.016347028 | 0.221242957 |
| H | 0.528255634 | 0.035571142 | 0.334259146 |
| H | 0.504722354 | 0.163162681 | 0.221184489 |
| H | 0.452110444 | 0.815461964 | 0.221966802 |
| H | 0.432650745 | 0.936583096 | 0.117423990 |
| H | 0.310133610 | 0.954450153 | 0.221084493 |
| H | 0.930227417 | 0.600033139 | 0.114220567 |
| H | 0.948999159 | 0.728228380 | 0.214619640 |
| H | 0.805074045 | 0.591055376 | 0.217229820 |
| H | 0.150307309 | 0.524926832 | 0.223849927 |
| H | 0.997285222 | 0.380142993 | 0.227081665 |
| H | 0.018440833 | 0.514886780 | 0.335585247 |
| H | 0.954463758 | 0.310168682 | 0.721113339 |
| H | 0.936631635 | 0.432584369 | 0.617405306 |
| H | 0.815459742 | 0.452129617 | 0.721923434 |
| H | 0.163155224 | 0.504786240 | 0.721169642 |
| H | 0.035516853 | 0.528405893 | 0.834218020 |
| H | 0.016318631 | 0.656362475 | 0.721149773 |
| H | 0.728244204 | 0.948968204 | 0.714678354 |
| H | 0.600117387 | 0.930282489 | 0.614241754 |
| H | 0.591059015 | 0.805050477 | 0.717202943 |
| H | 0.524964510 | 0.150284524 | 0.723950145 |
| H | 0.514817016 | 0.018318664 | 0.835620305 |
| H | 0.380155272 | 0.997281829 | 0.727062631 |
| Pb | 0.509483519 | 0.513945681 | 0.988568614 |
| Pb | 0.513937112 | 0.509463664 | 0.488568721 |
| Pb | 0.029281973 | 0.011051060 | 0.490216139 |
| Pb | 0.011075505 | 0.029293484 | 0.990216435 |
| I | 0.697940514 | 0.834399451 | 0.994920045 |
| I | 0.333252927 | 0.198560688 | 0.996934324 |
| I | 0.202813795 | 0.714353130 | 1.002368409 |
| I | 0.839417192 | 0.351903222 | 0.986264084 |
| I | 0.351885315 | 0.839386086 | 0.486303428 |
| I | 0.714336255 | 0.202785648 | 0.502384479 |
| I | 0.834389572 | 0.697920711 | 0.494903449 |
| I | 0.198547662 | 0.333234603 | 0.496899132 |
| I | 0.520646986 | 0.524765167 | 0.239976981 |
| I | 0.524762615 | 0.520638083 | 0.739975343 |
| I | 0.013998162 | 0.018889645 | 0.742089276 |
| I | 0.018867754 | 0.013982374 | 0.242088085 |

**I4/mcm**

| | | | |
|---|---|---|---|
| **CELL_PARAMETERS (alat=16.91193388)** | | | |
| | 0.953957482 | -0.000017614 | -0.000004625 |
| | 0.000016632 | 0.951906889 | 0.000014049 |
| | 0.000003284 | -0.000009893 | 1.410104436 |
| **ATOMIC_POSITIONS (crystal)** | | | |
| N | 0.9067084507 | 0.5963654811 | 0.2174935726 |
| N | 0.9067090441 | 0.4036338027 | 0.7174952812 |
| N | 0.5932901660 | 0.0963661947 | 0.2174944797 |
| N | 0.5932914023 | 0.9036348593 | 0.7174946488 |
| C | 0.0168580176 | 0.4901817484 | 0.2707744800 |
| C | 0.0168590746 | 0.5098172418 | 0.7707749254 |
| C | 0.4831413399 | 0.9901813314 | 0.2707747144 |
| C | 0.4831415565 | 0.0098178408 | 0.7707740213 |
| H | 0.1370755001 | 0.5200900600 | 0.2465642353 |
| H | 0.0044659261 | 0.5029317037 | 0.3570810249 |
| H | -0.0090443289 | 0.3683962012 | 0.2474621377 |
| H | 0.7902123158 | 0.5719310165 | 0.2378791806 |
| H | 0.9290396011 | 0.7141947712 | 0.2361371662 |
| H | 0.9156415332 | 0.5857832231 | 0.1354059756 |
| H | 0.1370764242 | 0.4799103082 | 0.7465636692 |
| H | -0.0090449048 | 0.6316024669 | 0.7474612749 |
| H | 0.0044669500 | 0.4970642623 | 0.8570814671 |
| H | 0.7902127422 | 0.4280679039 | 0.7378807446 |
| H | 0.9156423842 | 0.4142165119 | 0.6354077927 |
| H | 0.9290398516 | 0.2858043891 | 0.7361393276 |
| H | 0.3629241454 | 1.0200898781 | 0.2465637001 |
| H | 0.5090443966 | 0.8683960879 | 0.2474616872 |
| H | 0.4955345573 | 0.0029324919 | 0.3570811556 |
| H | 0.7097862271 | 0.0719312043 | 0.2378797848 |
| H | 0.5843555581 | 0.0857845151 | 0.1354070431 |
| H | 0.5709590720 | 0.2141953317 | 0.2361384413 |
| H | 0.3629237397 | -0.0200904938 | 0.7465639449 |
| H | 0.4955352645 | 0.9970656873 | 0.8570802879 |
| H | 0.5090450126 | 0.1316032609 | 0.7474605408 |
| H | 0.7097879544 | 0.9280698882 | 0.7378798090 |
| H | 0.5709594852 | 0.7858051990 | 0.7361379693 |
| H | 0.5843568584 | 0.9142193051 | 0.6354074011 |
| Pb | 0.0088496793 | 0.0107390236 | 0.0100531223 |
| Pb | 0.0088508902 | 0.9892599579 | 0.5100529300 |
| Pb | 0.4911489253 | 0.4892600777 | 0.5100518177 |
| Pb | 0.4911495382 | 0.5107395403 | 0.0100528250 |
| I | 0.1763874538 | 0.6880541264 | 0.0175115323 |
| I | 0.8113766029 | 0.3229015406 | 0.0153775678 |
| I | 0.3236115716 | 0.1880535917 | 0.0175118896 |
| I | 0.6886252560 | 0.8229008651 | 0.0153785878 |
| I | 0.6886226319 | 0.1770980310 | 0.5153808240 |
| I | 0.3236140861 | 0.8119477032 | 0.5175118194 |
| I | 0.8113783693 | 0.6770966841 | 0.5153809398 |
| I | 0.1763860412 | 0.3119477891 | 0.5175110478 |
| I | 0.9941951667 | 0.9997127488 | 0.2615205466 |
| I | 0.9941906896 | 0.0002890804 | 0.7615207823 |
| I | 0.5058114159 | 0.5002881571 | 0.7615203246 |
| I | 0.5058063673 | 0.4997154089 | 0.2615195561 |

# References


(S1) Stokes, H. T.; Hatch, D. M.; Campbell, B. FINDSYM. 2017; ISOTROPY Software Suite, iso.byu.edu.

(S2) Stokes, H. T.; Hatch, D. M. FINDSYM: program for identifying the space-group symmetry of a crystal. *J. Appl. Crystallogr.* **2005**, *38*, 237–238.

(S3) Brivio, F.; Frost, J. M.; Skelton, J. M.; Jackson, A. J.; Weber, O. J.; Weller, M. T.; Goni, A. R.; Leguy, A. M.; Barnes, P. R.; Walsh, A. Lattice dynamics and vibrational spectra of the orthorhombic, tetragonal, and cubic phases of methylammonium lead iodide. *Phys. Rev. B* **2015**, *92*, 144308.

(S4) Leppert, L.; Reyes-Lillo, S. E.; Neaton, J. B. Electric field-and strain-induced Rashba effect in hybrid halide perovskites. *J. Phys. Chem. Lett.* **2016**, *7*, 3683–3689.

(S5) Perdew, J. P.; Zunger, A. Self-interaction correction to density-functional approximations for many-electron systems. *Phys. Rev. B* **1981**, *23*, 5048–5079.

(S6) Perdew, J. P.; Wang, Y. Accurate and simple analytic representation of the electron-gas correlation energy. *Phys. Rev. B* **1992**, *45*, 13244.

(S7) Hamann, D. R. Optimized norm-conserving Vanderbilt pseudopotentials. *Phys. Rev. B* **2013**, *88*, 085117.

(S8) Van Setten, M.; Giantomassi, M.; Bousquet, E.; Verstraete, M. J.; Hamann, D. R.; Gonze, X.; Rignanese, G.-M. The PseudoDojo: Training and grading a 85 element optimized norm-conserving pseudopotential table. *Comput. Phys. Commun.* **2018**, *226*, 39–54.

(S9) Pérez-Osorio, M. A.; Lin, Q.; Phillips, R. T.; Milot, R. L.; Herz, L. M.; Johnston, M. B.; Giustino, F. Raman spectrum of the organic–inorganic halide perovskite

$CH_3NH_3PbI_3$ from first principles and high-resolution low-temperature Raman measurements. *J. Phys. Chem. C* **2018**, *122*, 21703–21717.

(S10) Mouhat, F.; Coudert, F.-X. Necessary and sufficient elastic stability conditions in various crystal systems. *Phys. Rev. B* **2014**, *90*, 224104.
